# Supplementary material for: HeLM: Highlighted Evidence augmented Language Model for Enhanced Table-to-Text Generation
Source: arXiv:2311.08896 source file (2024-04-27)
Supplement: Supplementary file 1 [file s7_appendix.tex]

\newpage
\begin{figure*}[ht]
    \centering
    \includegraphics[width=1.0\textwidth]{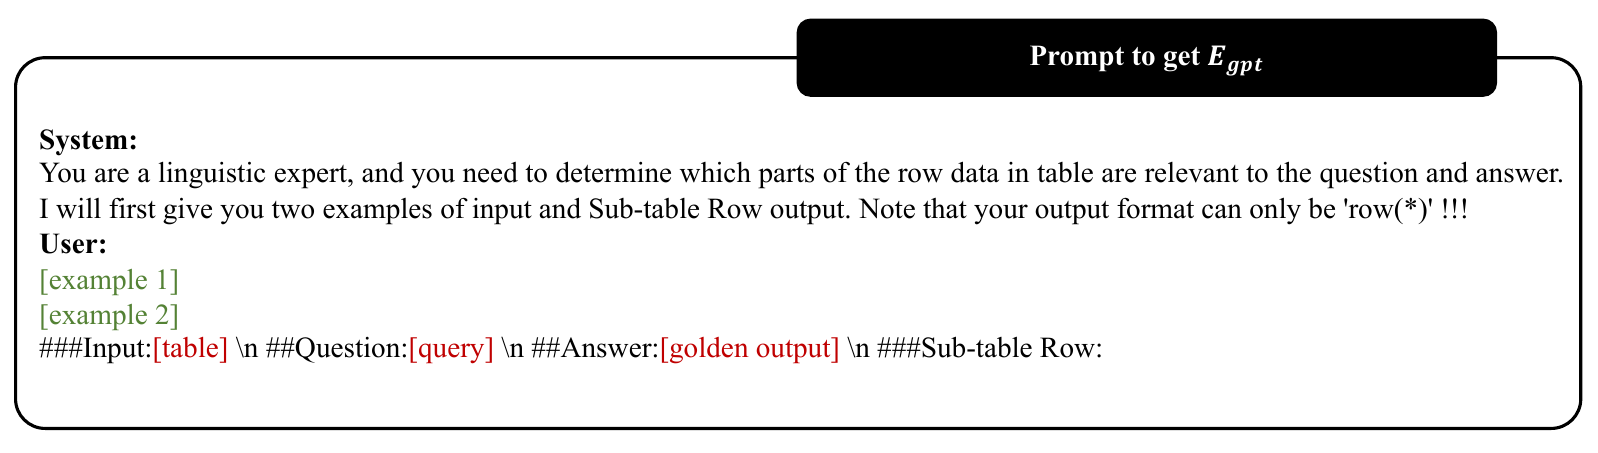}
    \caption{The prompt used to obtain $E_{gpt}$ using GPT-3.5-trubo. The content within the green brackets represents two examples used for few-shot learning. The inputs such as tables, queries, etc., within the red brackets, can be replaced according to specific input requirements.}
    \vspace*{0.4cm}
    \label{fig:prompt_egpt}
\end{figure*}
% 这是使用 GPT3.5-trubo 来获得 Egpt 所使用的 prompt。绿色括号里的内容代表来进行 fewshot-learning 的两个例子。红色括号中的输入 table，query 等可根据具体的输入替换。

\appendix

\section{Prompt Design}
\label{sec:appendix}
\noindent \textbf{Prompt to get} $E_{gpt}$:  To achieve better results, we incorporate two examples of input-output pairs within the prompt to help LLMs understand the output format. Additionally, we include the golden summary $\mathcal{Y}$ to guide a better identification of evidence. 
% 为了得到好的结果，我们在 prompt 里面添加了输入输出的例子让 LLMs 来了解输出的格式，同时加入了 golden summmary $\mathcal{Y}$ 来引导更好的找到 evidence。
The details of the prompt template for obtaining $E_{gpt}$ can be found in Figure \ref{fig:prompt_egpt}. 
% 获取 $E_{gpt}$ 的 prompt 模版细节见 figure \ref{fig:prompt_egpt}.
Additionally, the two samples used in the prompt can be found in Figure \ref{fig:prompt_example}.
% 另外，Prompt 里使用的两个 samples 见 figure 4.
\input{latex/miscs/figure_prompt_hellama}

\noindent \textbf{Prompt of reasoner and summarizer}
% 在 HeLM 中，table reasoner 和 summarizer 都使用了 LLMs，所以需要构建输入的 prompt text。figure 5 展示了在 HeLM 的两个 LLMs 所用到的 prompt 模版。
% \input{latex/miscs/figure_prompt_hellama}
In HeLM, both the table reasoner and summarizer utilize LLMs, necessitating the construction of input prompt text. Figure \ref{fig:prompt_helm} displays the prompt templates used for the two components in HeLM. 
% 在推理的时候，prompt 里 ###Output 后面置空。
During inference, leave the area after ``\#\#\#Output'' in the prompt blank.

\section{Code libraries}
% HeLM 使用了 pytorch 深度学习框架，加载的是 huggingface 提供的模型，parameter-efficient finetuning 使用的是 PEFT 包。模型的训练框架是在 LLM-fintuning HUB 的基础上进行的修改。
HeLM utilizes the \textit{PyTorch} deep learning framework, loading models provided by \textit{Huggingface}, and utilizes the \textit{PEFT} package for parameter-efficient fine-tuning. The training framework of the model is modified based on the \textit{LLM-finetuning HUB}.
\begin{figure}[hp]
\centering

\includegraphics[width=\linewidth]{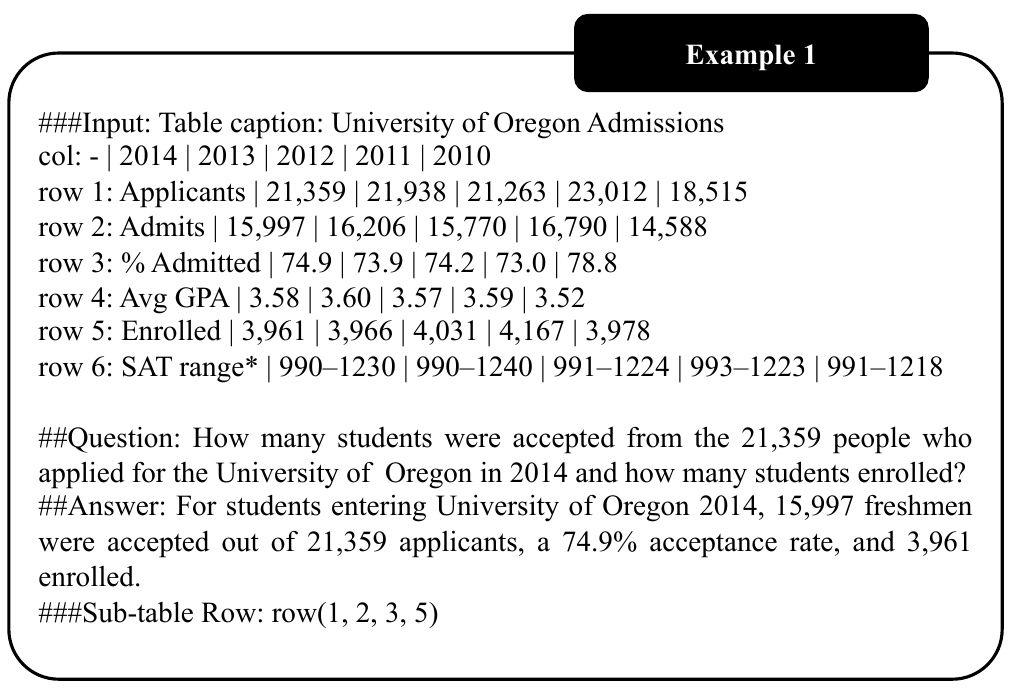} \\
\includegraphics[width=\linewidth]{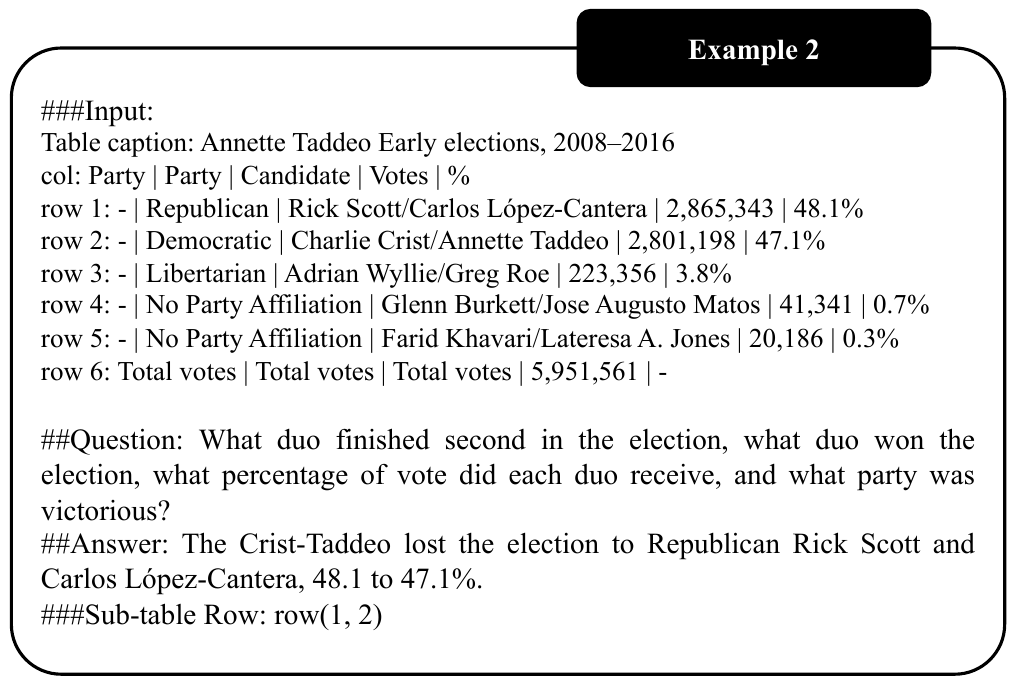}
\caption{Two examples used in figure \ref{fig:prompt_egpt}}
\vspace*{0.4cm}
\label{fig:prompt_example}
\end{figure}
